# Supplementary material for: Network Traffic Characteristics of IoT Devices in Smart Homes
Source: arXiv:2109.01855 source file (2021-09-04)
Supplement: Supplementary file 1 [file 10_additional.tex]

\section{Additional Figures}
\begin{figure*}[th]
\centering
\subcaptionbox{Flow duration (TCP and UDP) of IoT devices \label{fig:flow_duration_iot}}[0.48\linewidth]
    {\includegraphics[width=0.48\textwidth]{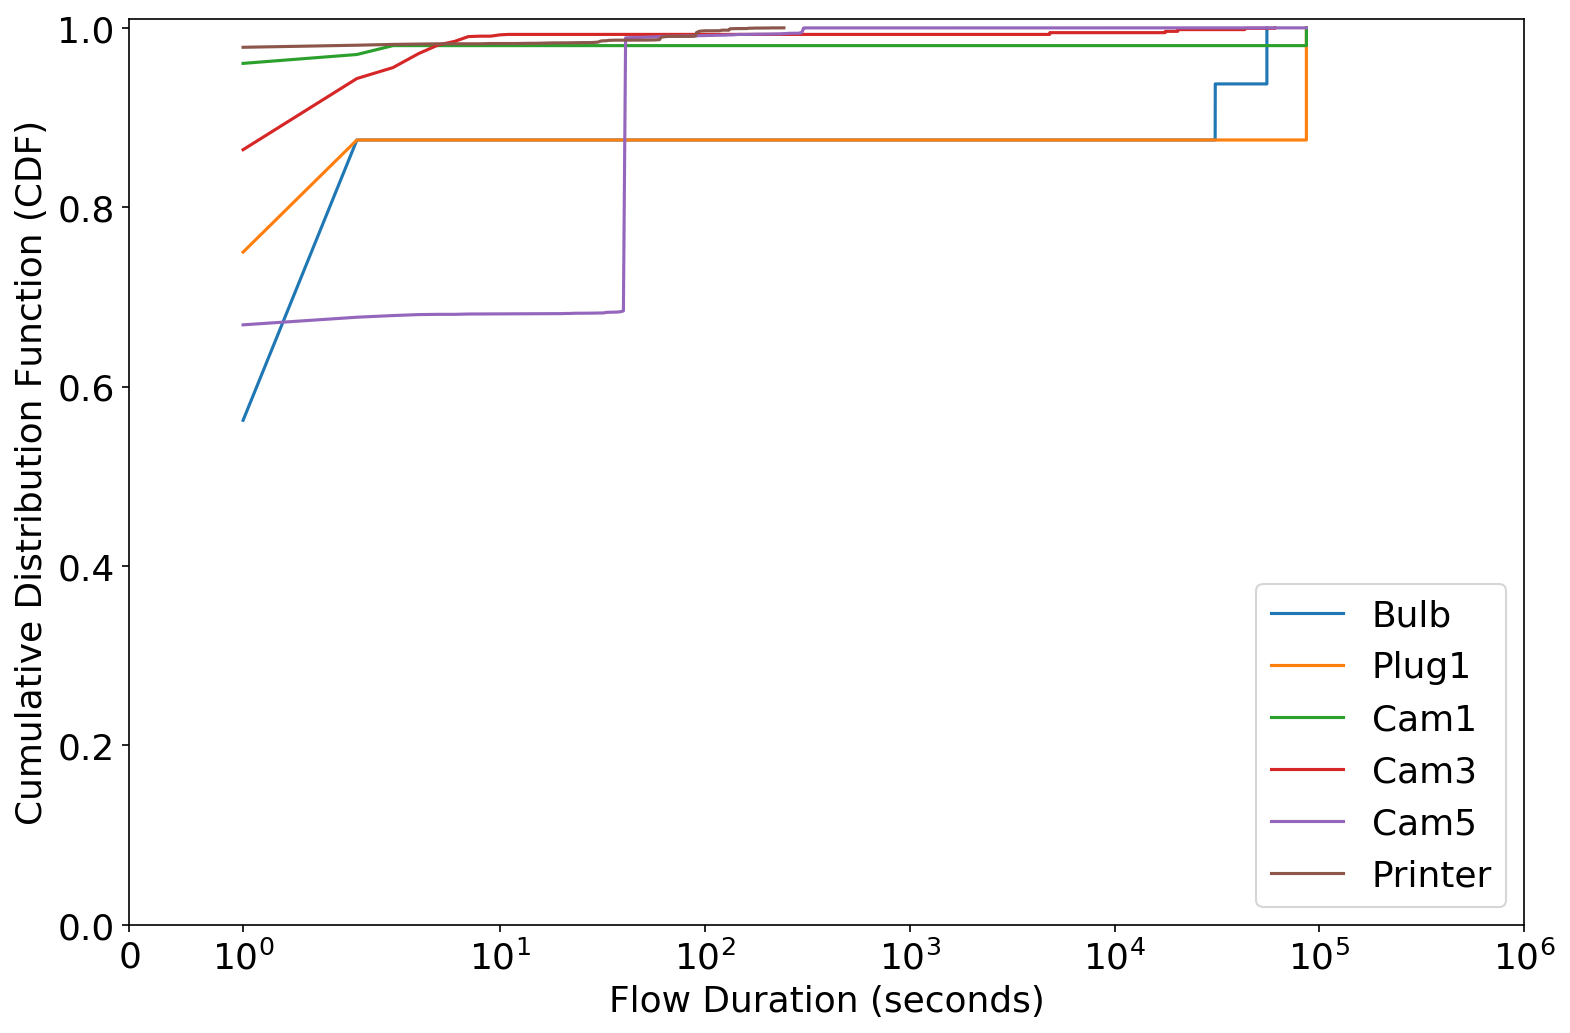}}
\hfill
\subcaptionbox{Flow duration (TCP and UDP) of non-IoT devices \label{fig:flow_duration_noniot}}[0.48\linewidth]
    {\includegraphics[width=0.48\textwidth]{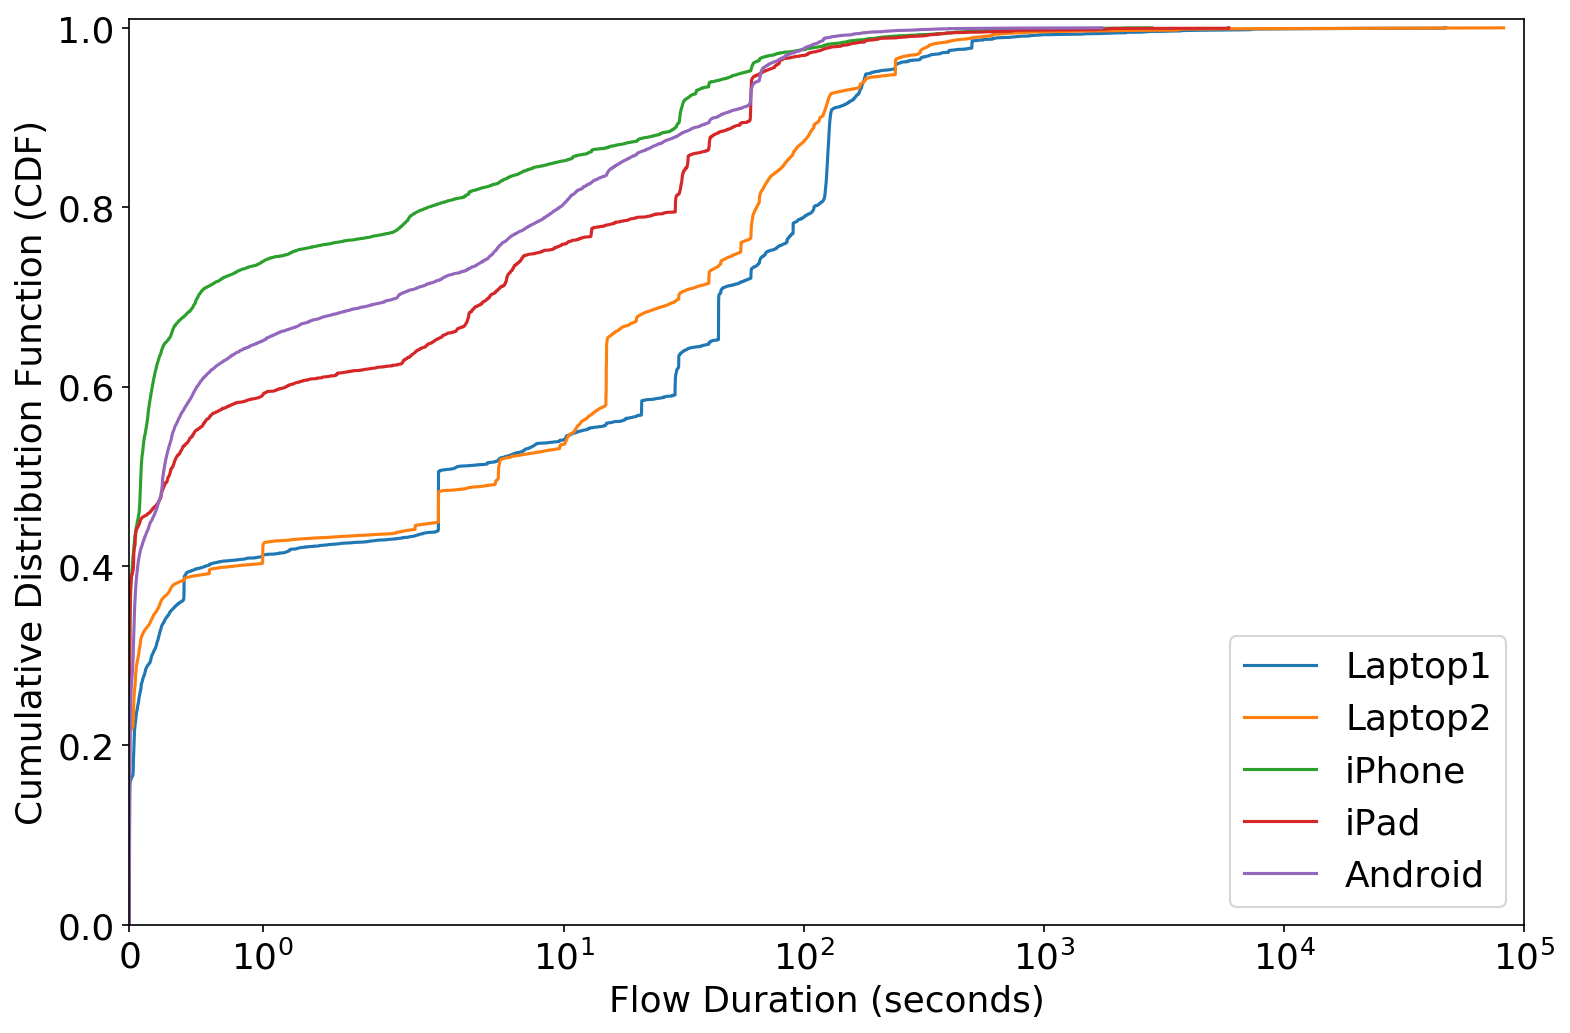}}
  \caption{Flow duration for IoT and non-IOT devices.}
\label{fig:flow-durations}
\end{figure*}

Figures~\ref{fig:flow_duration_iot} and~\ref{fig:flow_duration_noniot} shows the flow duration of a few representative IoT and non-IoT devices. In these two figures, a flow can be either a TCP or UDP flow. First we note that a large percentage of flows have very short flow durations for all IoT devices. Non-IoT devices also have a large number of flows with short flow durations. However, this percentage is lower in non-IoT devices. Second, we note that a number of IoT devices have a few concentrated flow durations. For example, about $30\%$ of the Cam5 flows have a flow duration of $120$ seconds. In contrast, as we can see from Figure~\ref{fig:flow_duration_noniot} that non-IoT devices do not have this kind of concentrated flow durations. The durations of non-IoT flows are more spread out. 

\begin{figure*}[th]
\centering
\subcaptionbox{Flow size (TCP and UDP) for IoT devices \label{fig:flow-bytes-iot}}[0.48\linewidth]
    {\includegraphics[width=0.48\textwidth]{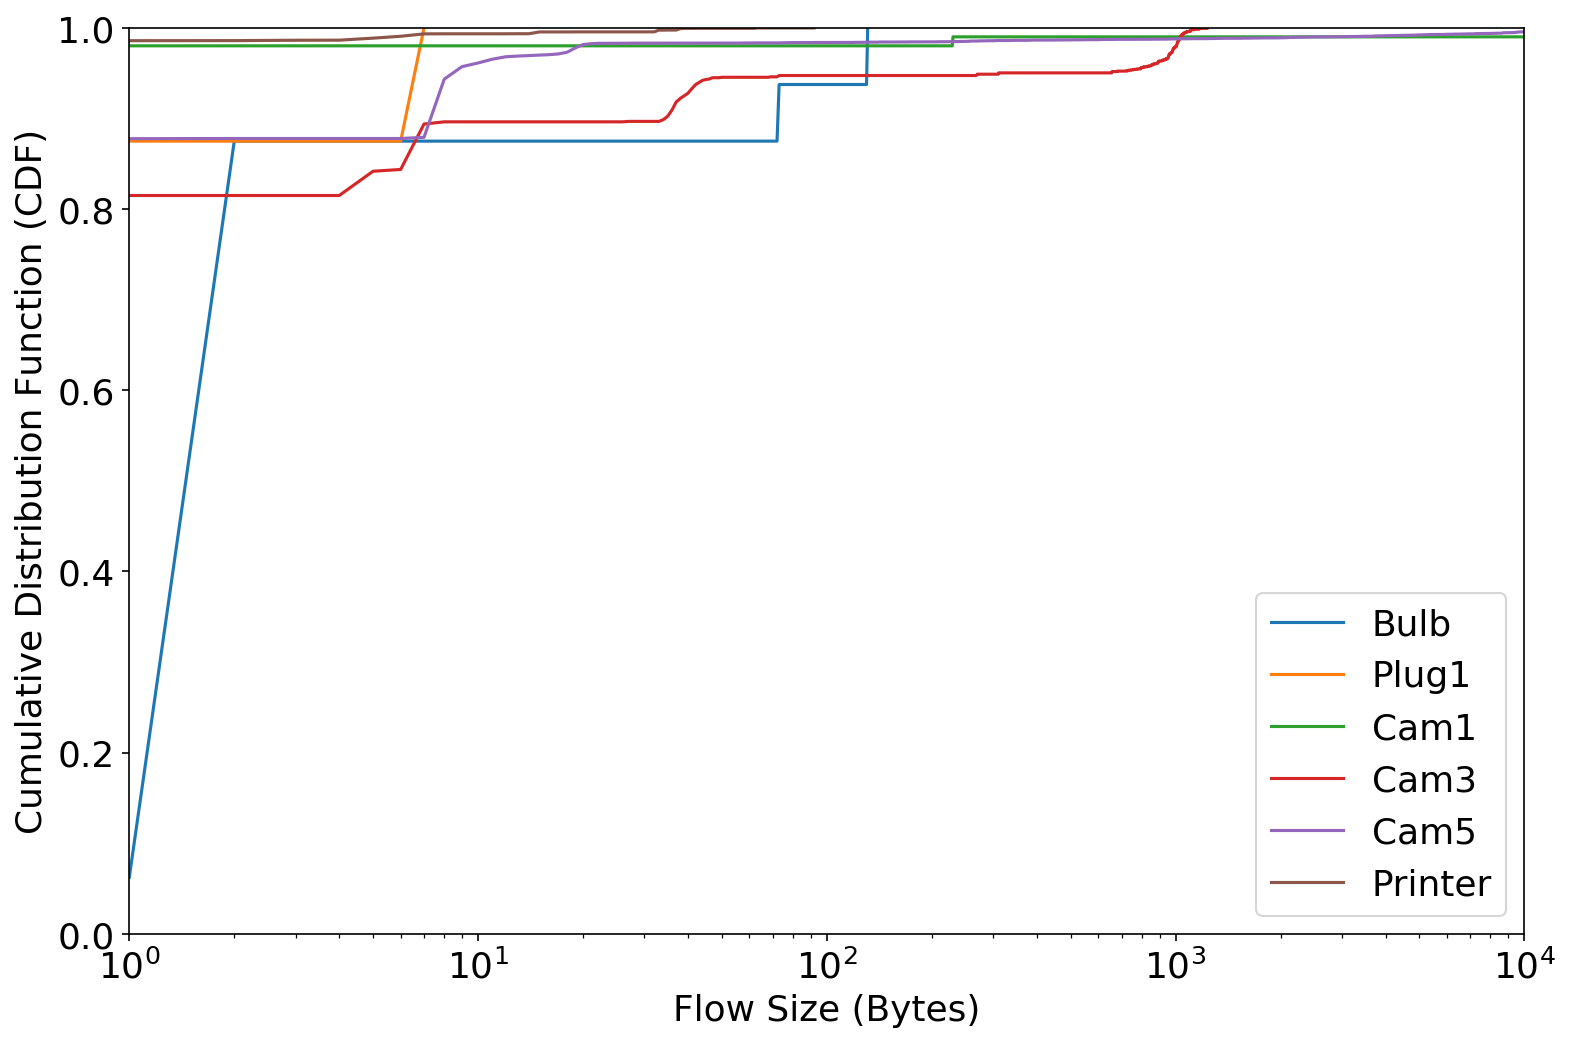}}
\hfill
\subcaptionbox{Flow size (TCP and UDP) for non-IoT devices \label{fig:flow-bytes-noniot}}[0.48\linewidth]
    {\includegraphics[width=0.48\textwidth]{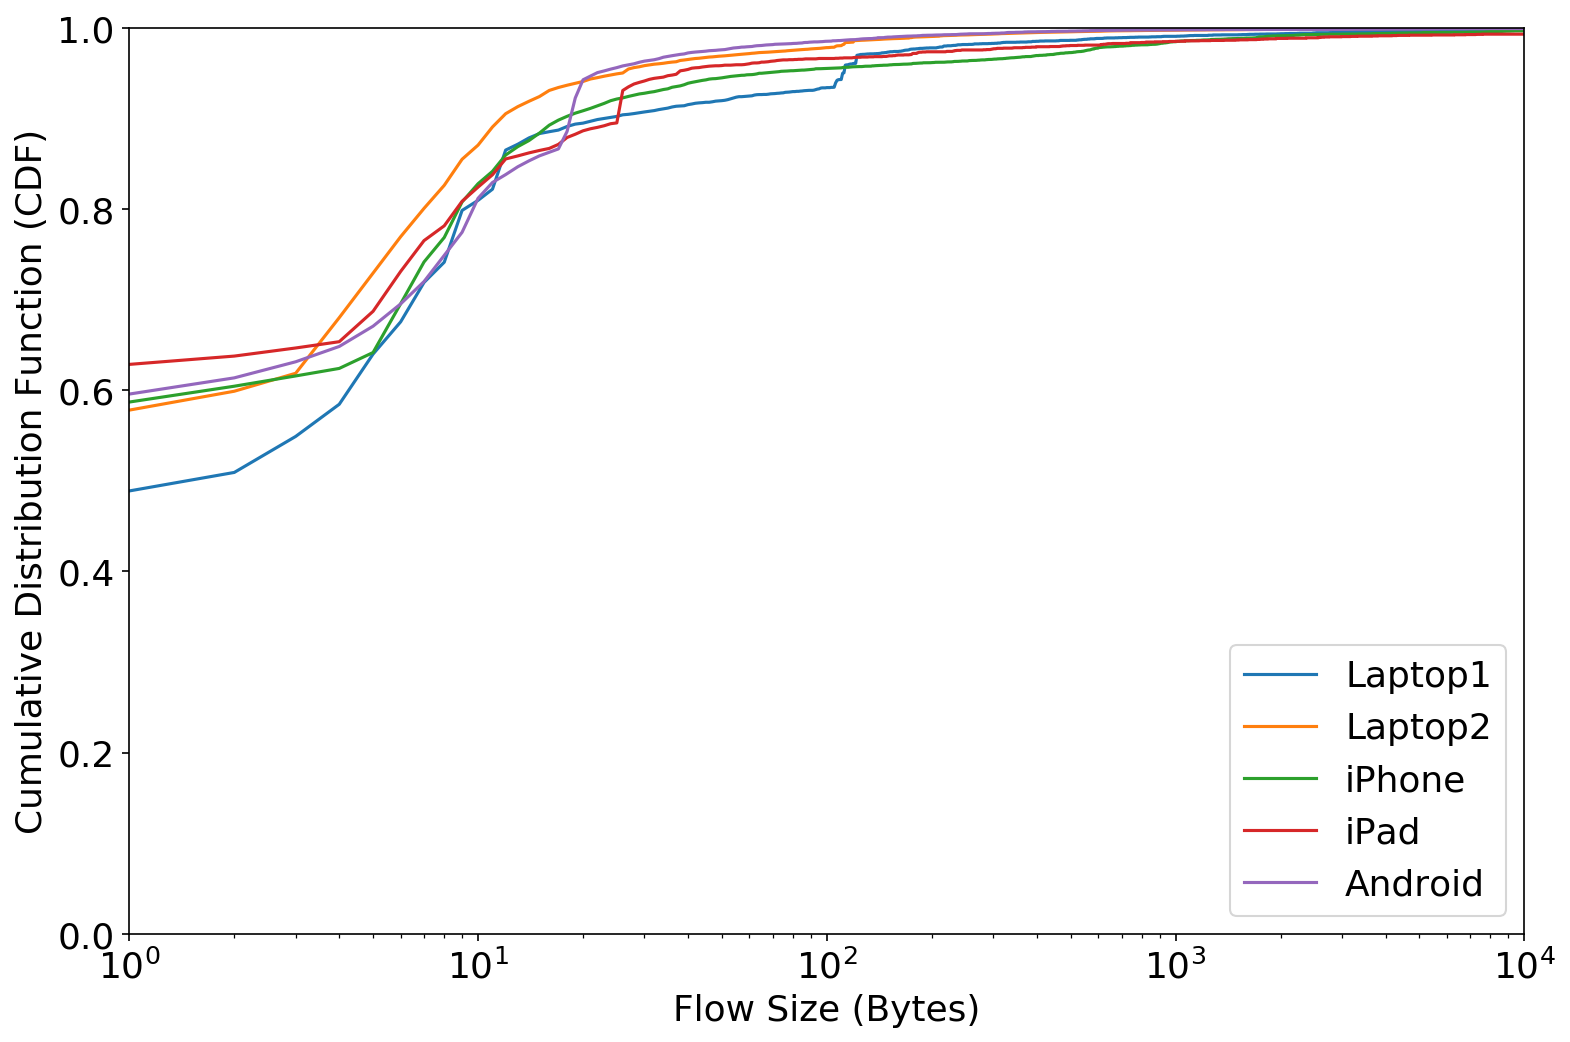}}
\caption{Flow size for IoT and non-IOT devices.}
\label{fig:flow-bytes}
\end{figure*}

Figure~\ref{fig:flow-bytes-iot} shows the amount of traffic of flows of IoT devices. From the figure we can see that most of IoT devices only generate a small amount of traffic. For example, close to $90\%$ of flows of all IoT devices generated less than $10$ bytes of data traffic. Figure~\ref{fig:flow-bytes-noniot} shows the amount of traffic of flows of non-IoT devices. From the figure we can see that, on average, non-IoT devices have larger flows. For example, only less than $70\%$ of flows of all non-IoT devices generated less than $10$ bytes of data traffic.

\begin{figure*}[!h]
%\subcaptionbox{Subcaption A}
\begin{subfigure}[b]{0.48\textwidth}
    \includegraphics[width=\textwidth]{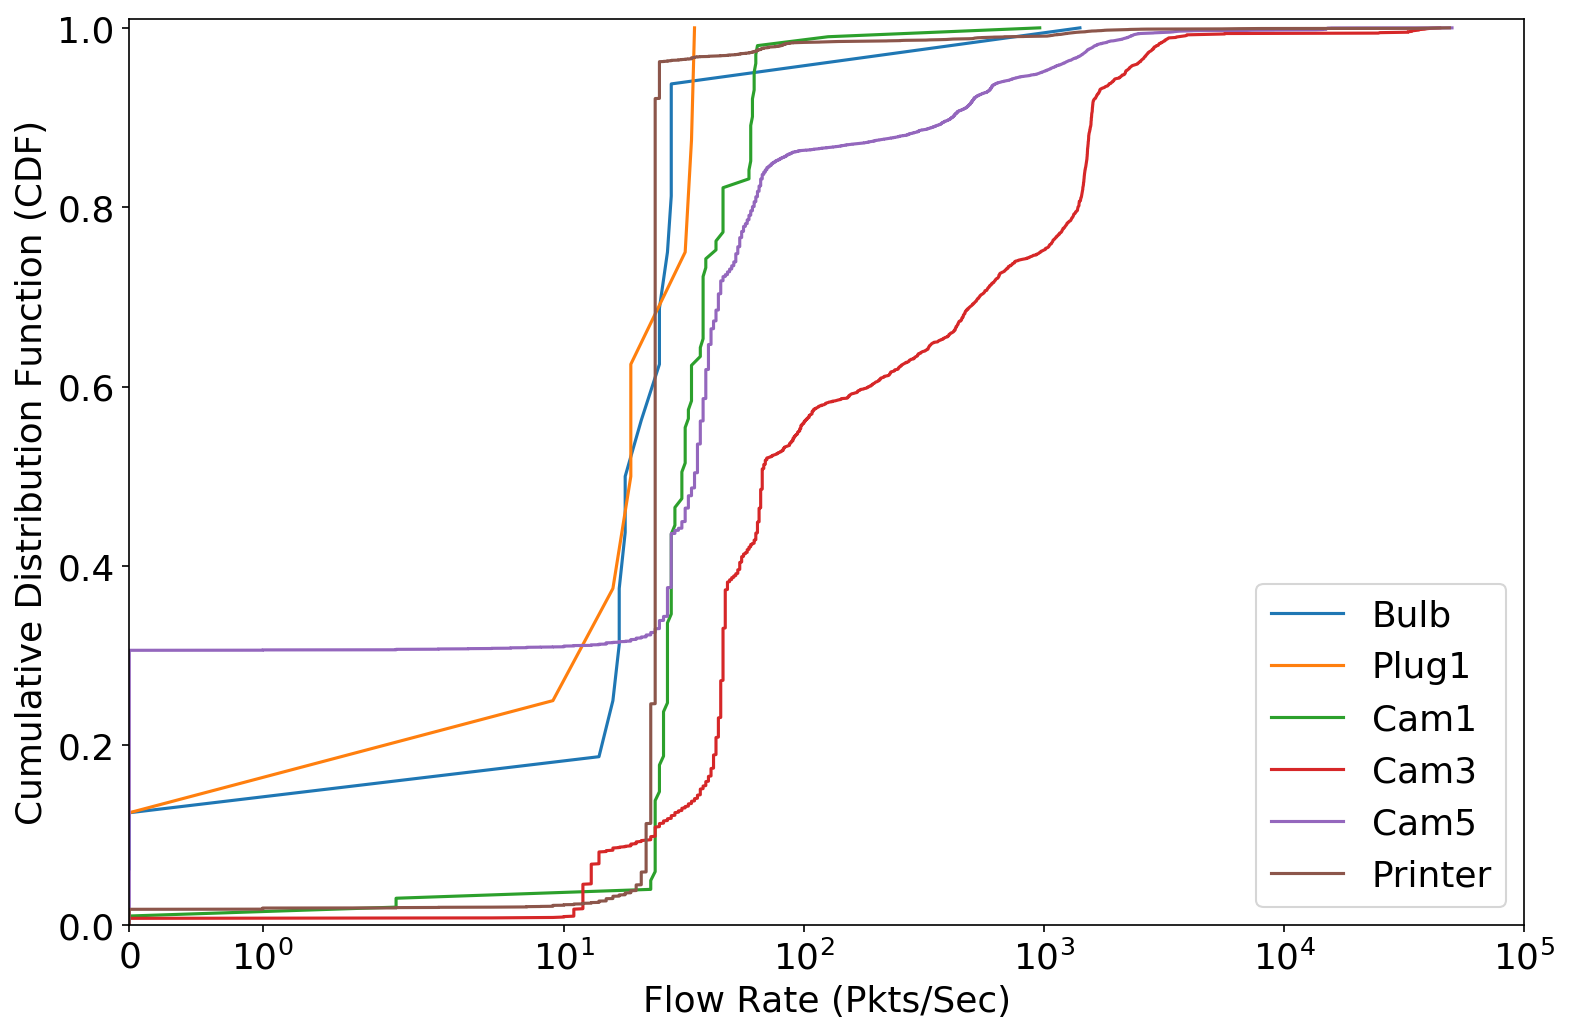}
    \caption{IoT devices}
    \label{fig:flow-rate-pkts-iot}
\end{subfigure}
\hfill
\begin{subfigure}[b]{0.48\textwidth}
    \includegraphics[width=\textwidth]{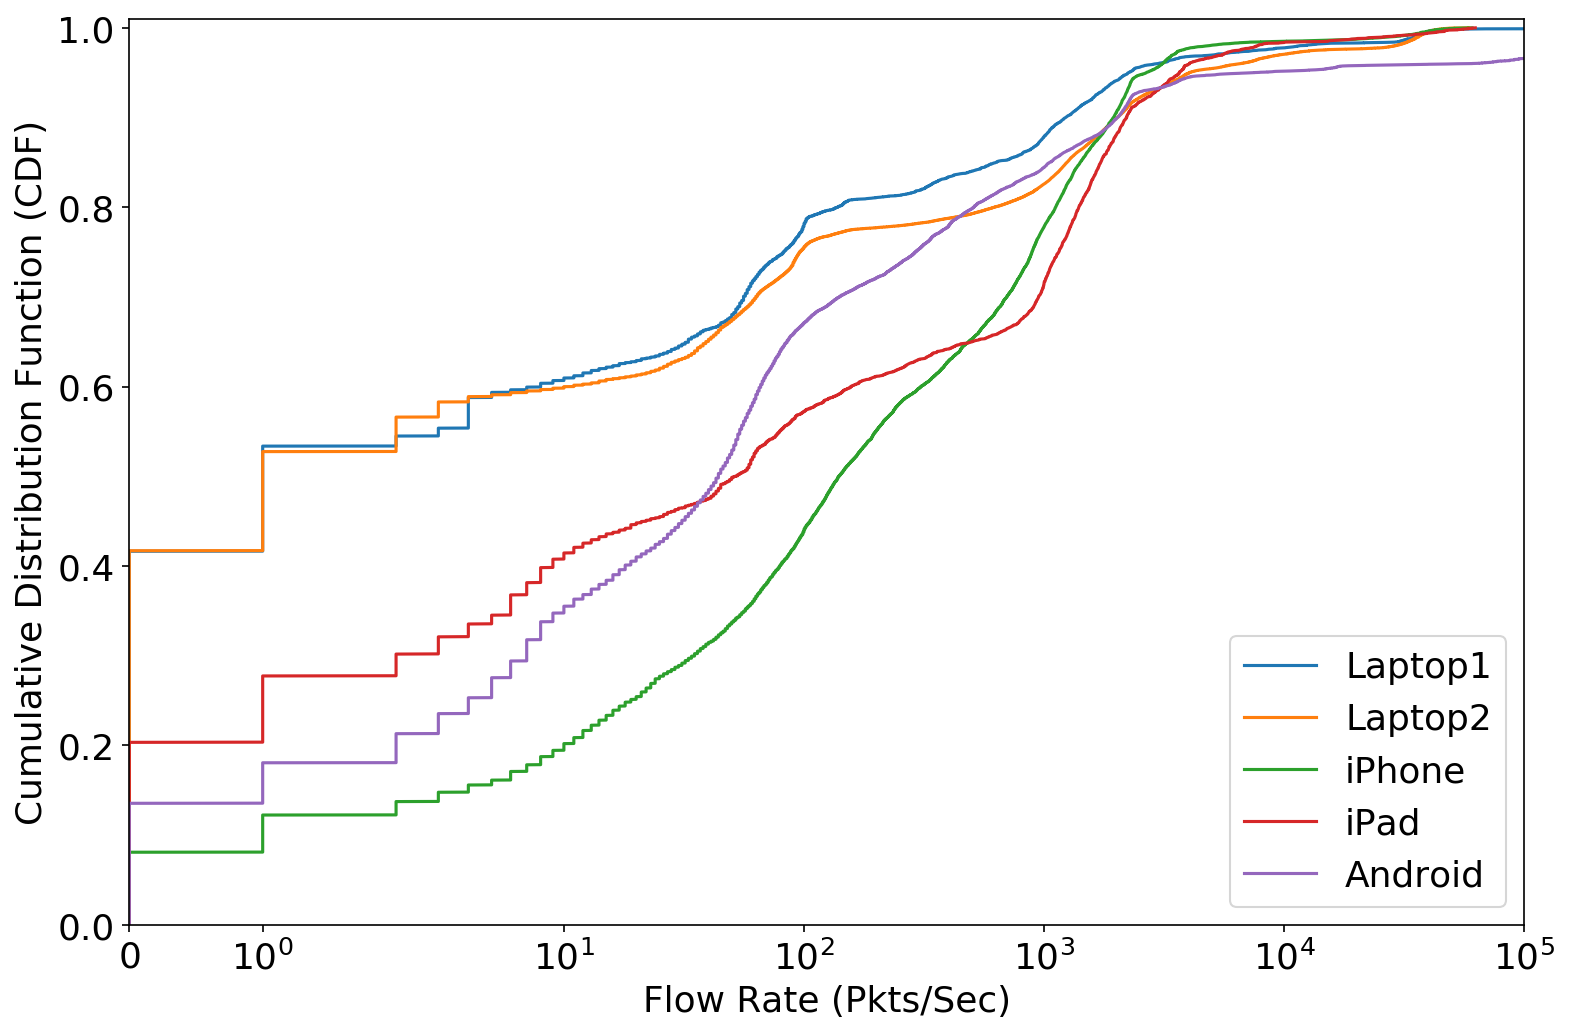}
    \caption{Non-IoT devices}
    \label{fig:flow-rate-pkts-noniot}
\end{subfigure}
\caption{TCP+UDP Flow rate (packets/second).}
\label{fig:flow-rate-pkts}
\end{figure*}

\begin{figure*}[!h]
\begin{subfigure}[b]{0.48\textwidth}
    \includegraphics[width=\textwidth]{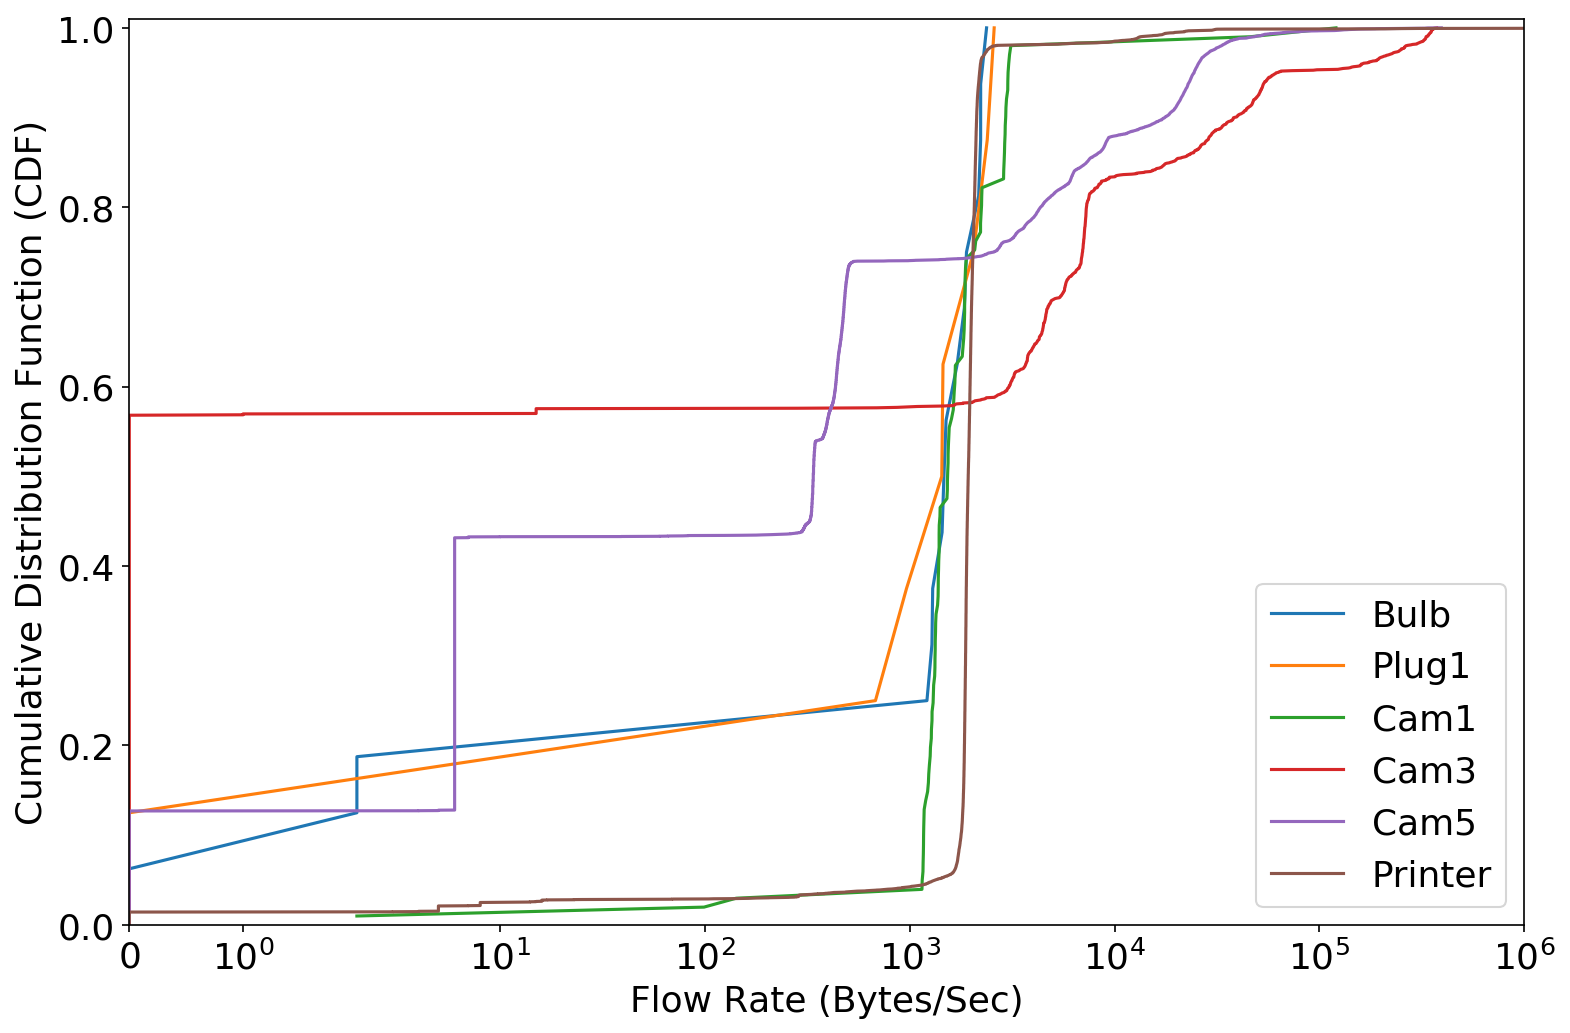}
    \caption{IoT devices}
    \label{fig:flow-rate-bytes-iot}
\end{subfigure}
\hfill
\begin{subfigure}[b]{0.48\textwidth}
    \includegraphics[width=\textwidth]{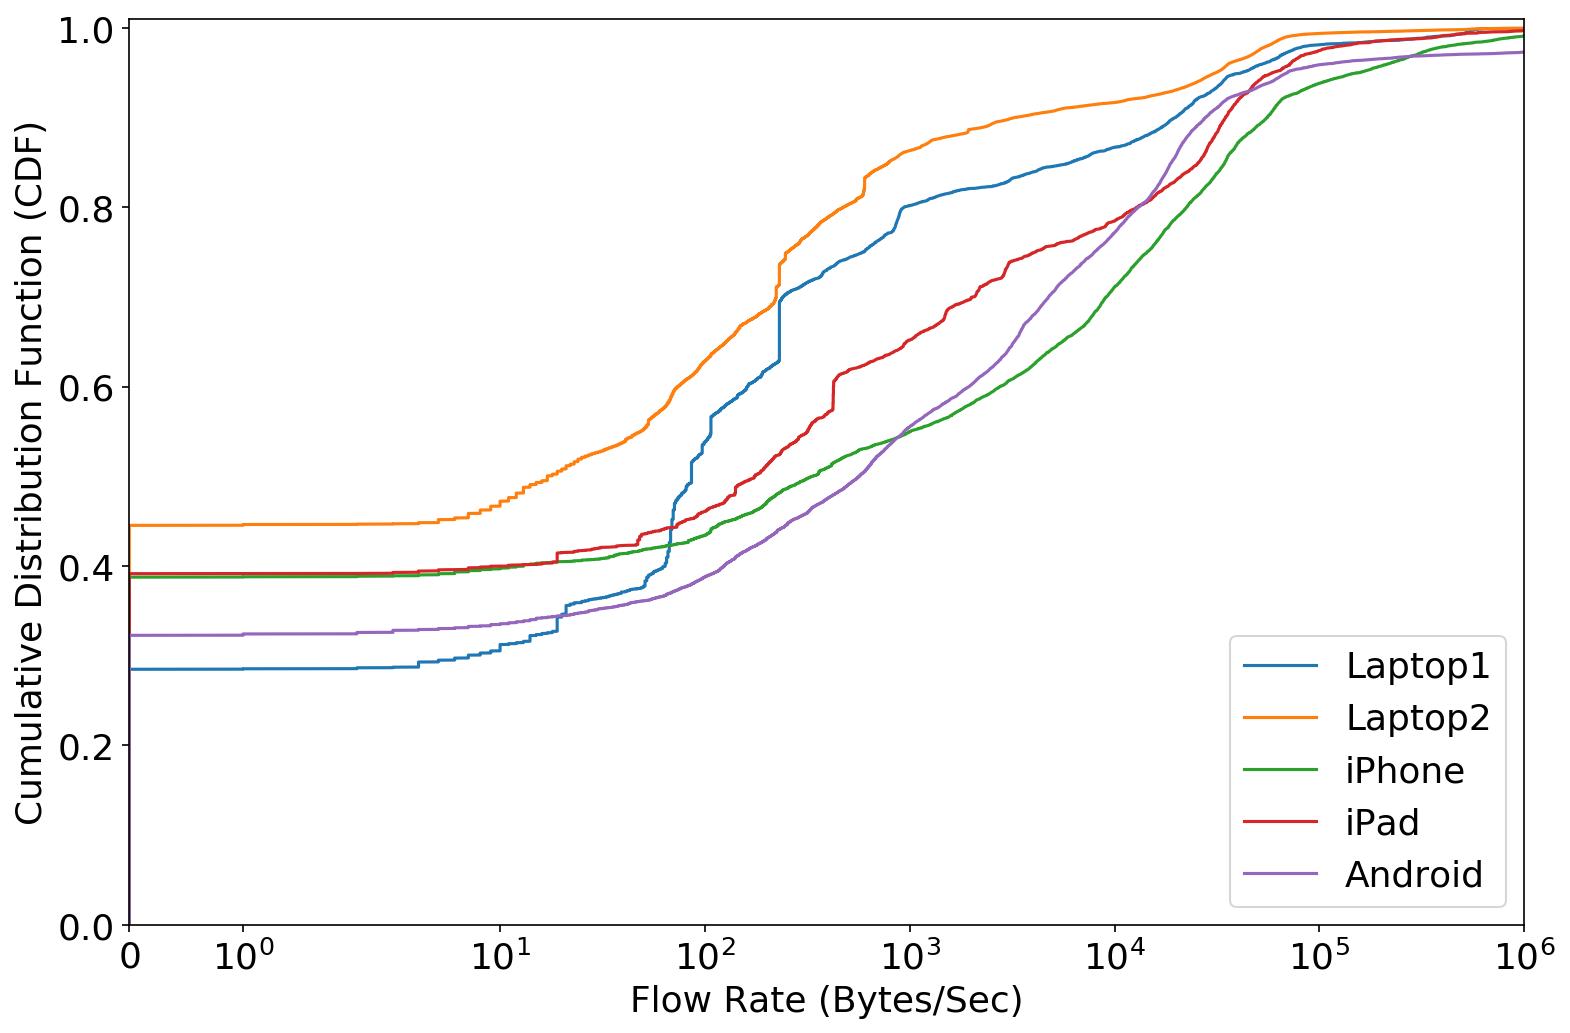}
    \caption{Non-IoT devices}
    \label{fig:flow-rate-bytes-noniot}
\end{subfigure}

\caption{TCP+UDP Flow rate (bytes/second).}
\label{fig:flow-rate-bytes}
\end{figure*}

\begin{figure*}[th]
\centering
\subcaptionbox{IoT devices \label{fig:active-flows-iot}}[0.48\linewidth]
    {\includegraphics[width=0.48\textwidth]{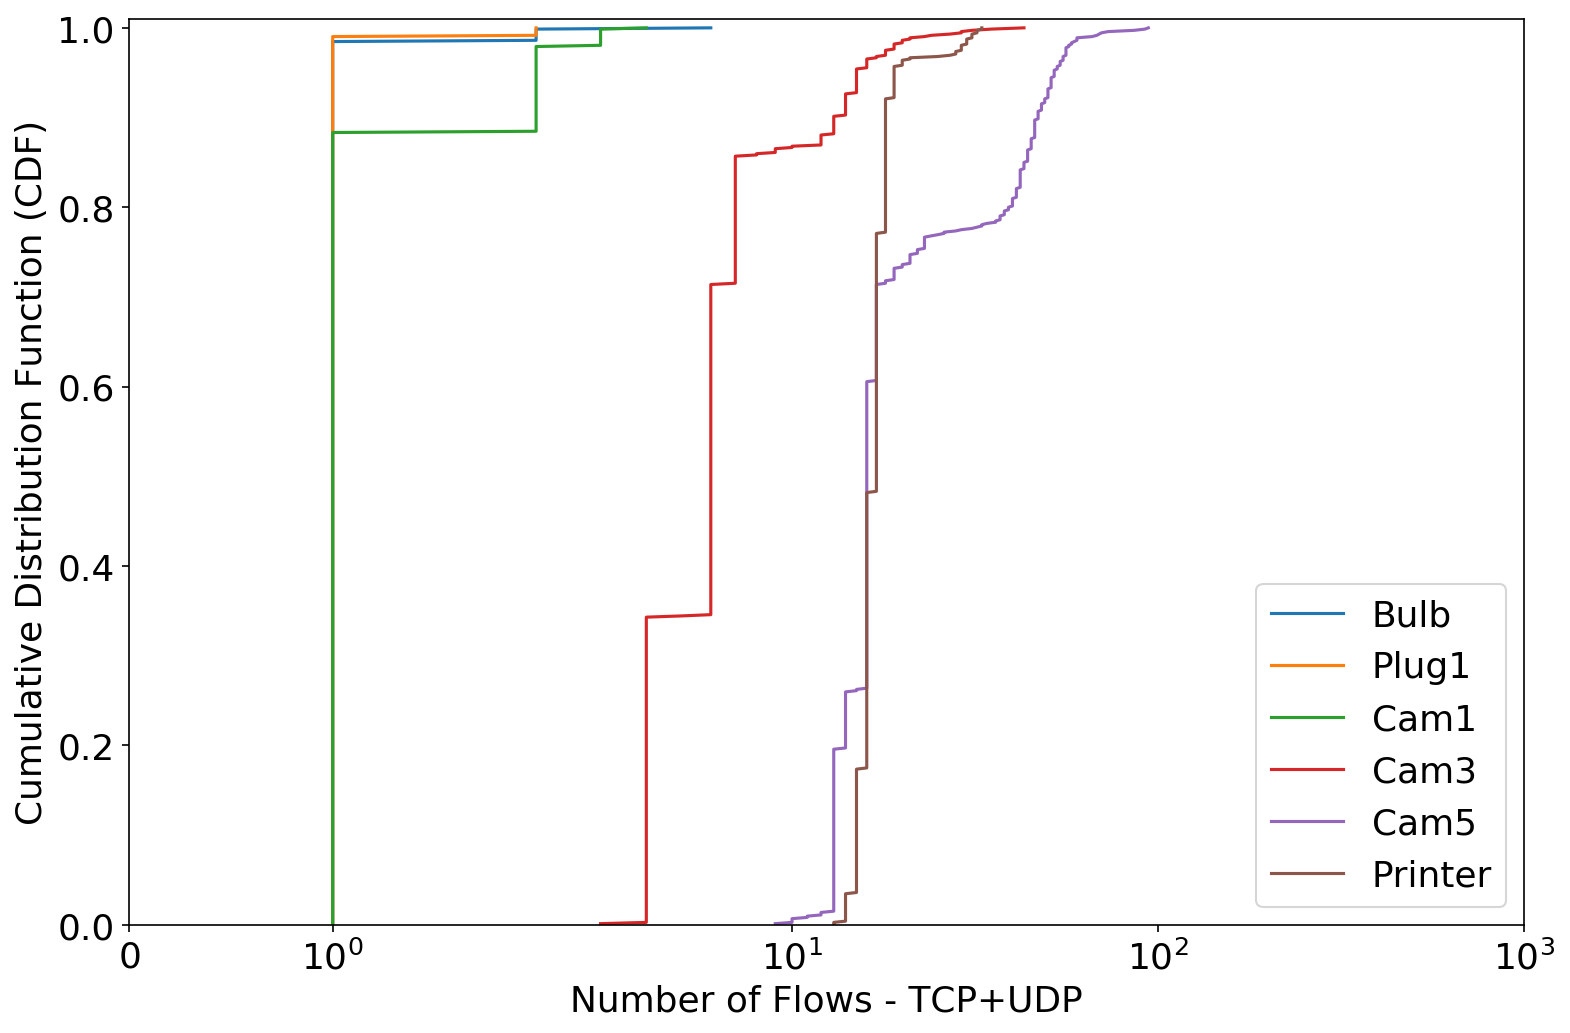}}
\hfill
\subcaptionbox{non-IOT devices \label{fig:active-flows-noniot}}[0.48\linewidth]
    {\includegraphics[width=0.48\textwidth]{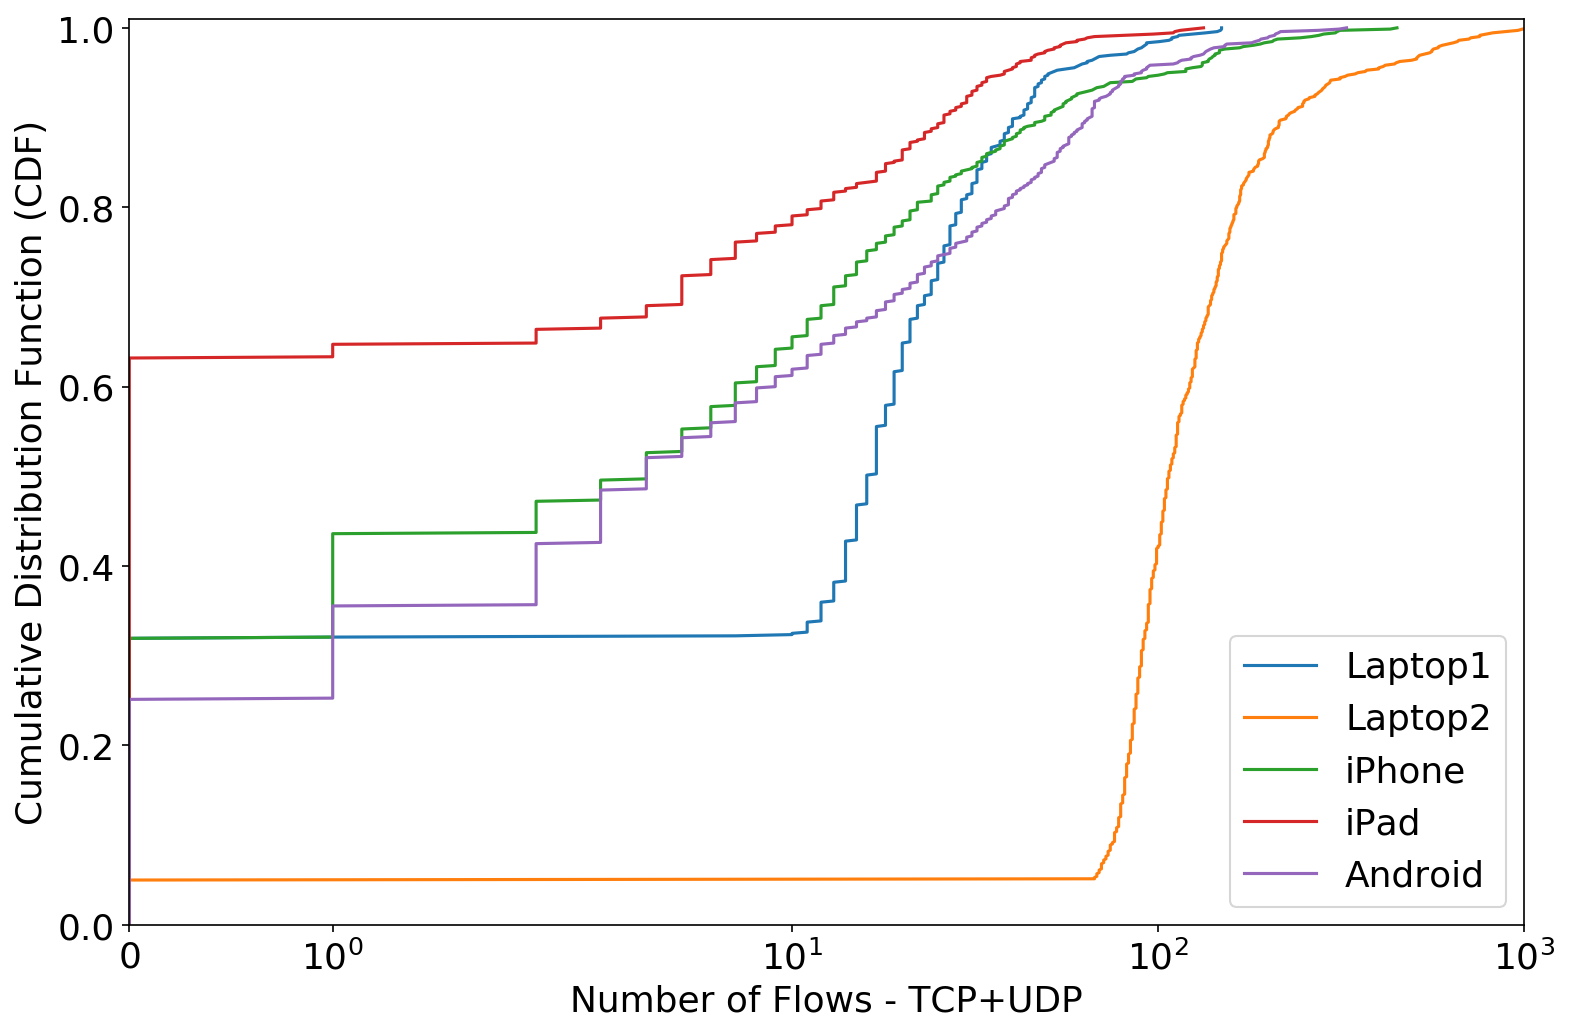}}
\caption{Number of Flows (TCP+UDP) for IoT and non-IOT devices at time intervals.}
\label{fig:active-flows}
\end{figure*}
